# Supplementary material for: Novel Hybrid-Learning Algorithms for Improved Millimeter-Wave Imaging Systems
Source: arXiv:2306.15341 source file (2023-06-27)
Supplement: Supplementary file 1 [file appendixX.tex]

\chapter{Spatial Fourier Transform and Relations}
\label{app:spatial_ft}
Neglecting amplitude terms, the \mbox{1-D}, \mbox{2-D} and \mbox{3-D} spatial Fourier transforms can be defined as \cite{yanik2019sparse}
\begin{equation}
\label{eq:ft1D}
    \text{FT}_{\text{1D}}^{(u)} \left[ s(u) \right] = S(k_u) = \int s(u) e^{-jk_u u}du,
\end{equation}

\begin{equation}
\label{eq:ft2D}
    \text{FT}_{\text{2D}}^{(u,v)} \left[ s(u,v) \right] = S(k_u,k_v) = \iint s(u,v) e^{-j(k_u u + k_v v)}du dv,
\end{equation}

\begin{equation}
\label{eq:ft3D}
    \text{FT}_{\text{3D}}^{(u,v,w)} \left[ s(u,v,w) \right] = S(k_u,k_v,k_w) = \iiint s(u,v,w) e^{-j(k_u u + k_v v + k_w w)}du dv dw.
\end{equation}

Similarly, the \mbox{1-D}, \mbox{2-D} and \mbox{3-D} inverse spatial Fourier transforms can be expressed as
\begin{equation}
\label{eq:ift1D}
    \text{IFT}_{\text{1D}}^{(k_u)} \left[ S(k_u) \right] = s(u) = \int S(k_u) e^{jk_u u}du,
\end{equation}

\begin{equation}
\label{eq:ift2D}
    \text{IFT}_{\text{2D}}^{(k_u,k_v)} \left[ S(k_u,k_v) \right] = s(u,v) = \iint S(k_u,k_v) e^{j(k_u u + k_v v)}du dv,
\end{equation}

\begin{equation}
\label{eq:ift3D}
    \text{IFT}_{\text{3D}}^{(k_u,k_v,k_w)} \left[ S(k_u,k_v,k_w) \right] = s(u,v,w) = \iiint S(k_u,k_v,k_w) e^{j(k_u u + k_v v + k_w w)}du dv dw.
\end{equation}

A shift in the spatial domain results in a corresponding phase shift in the spatial spectral domain. The example given here is in the \mbox{3-D} spatial domain but holds true for the \mbox{2-D} and \mbox{1-D} cases also:
\begin{equation}
\label{eq:ft_shiftForward}
    \text{FT}_{\text{3D}}^{(u,v,w)} \left[ s(u - u_0,v - v_0,w - w_0) \right] = e^{-j(k_u u_0 + k_v v_0 + k_w w_0)}S(k_u,k_v,k_w).
\end{equation}

Similarly, a shift in the spatial spectral domain results in a phase shift in the spatial domain:

\begin{equation}
\label{eq:ft_shiftInverse}
    \text{IFT}_{\text{3D}}^{(k_u,k_v,k_w)} \left[ S(k_u - k^u_0,k_v - k^v_0,k_w - k^w_0) \right] = e^{j(k_u u_0 + k_v v_0 + k_w w_0)}s(u,v,w).
\end{equation}

These spatial Fourier transform definitions and relations are useful in deriving the reconstruction algorithms discussed in the subsequent appendices.
