# Supplementary material for: Novel Hybrid-Learning Algorithms for Improved Millimeter-Wave Imaging Systems
Source: arXiv:2306.15341 source file (2023-06-27)
Supplement: Supplementary file 2 [file appendixY.tex]

\chapter{Method of Stationary Phase}
\label{app:msp}
As discussed in \cite{cook2012radar,papoulis1968systems,mcclure2016multidimensional}, the general form of the \mbox{$n$-dimensional} Method of Stationary Phase (MSP) can be expressed as the following. A rigorous mathematical perspective is offered in \cite{mcclure2016multidimensional}, whereas our discussion does not comprehensively address the underlying assumptions and constraints. Rather, this section is meant to serve as a resource to researchers and engineers to apply the results of the MSP approximation to near-field spherical wave decomposition problems.

Given an oscillatory integral with a wide phase variation of the form
\begin{equation}
    I(\mathbf{x}) = \int g(\mathbf{x}) e^{jf(\mathbf{x})}d\mathbf{x}, \quad \mathbf{x} \in \mathbb{R}^n,
\end{equation}
where $f(\mathbf{x})$ is assumed to be twice-continuously differentiable, the major contribution to the quantity $I(\mathbf{x})$ is from the stationary points, $\mathbf{x}_0$, which are calculated by
\begin{equation}
    \nabla f(\mathbf{x}) |_{\mathbf{x} = \mathbf{x}_0} = 0
\end{equation}

Thus, the integral can be approximated by
\begin{equation}
    I(\mathbf{x}) \approx \frac{g(\mathbf{x}_0)}{\sqrt{\det\mathbf{A}}} e^{j f(\mathbf{x}_0)},
\end{equation}
where $\mathbf{x}_0$ is the set of stationary points and $\mathbf{A}$ is the Hessian matrix of $f(\mathbf{x})$ evaluated at $\mathbf{x}_0$ and defined as
\begin{equation}
    \mathbf{A} = \left( \frac{\partial^2f(\mathbf{x})}{\partial x_i \partial x_j} \right) \biggr\rvert_{\mathbf{x} = \mathbf{x}_0}.
\end{equation}

For the derivations required in this article, we can limit $n$ to 1 or 2 dimensions. 
\section{\mbox{1-D} Method of Stationary Phase}
\label{subsec:msp_1D}
The \mbox{1-D} MSP can be written as the following. The following integral with the same assumptions as the MSP,
\begin{equation}
    I(u) = \int g(u) e^{j f(u)} du,
\end{equation}
can be approximated as 
\begin{equation}
\label{eq:msp_1D}
    I(u) \approx \frac{g(u_0)}{\sqrt{f''(u_0)}} e^{j f(u_0)},
\end{equation}
where $u_0$ is the stationary point calculated by
\begin{equation}
\label{eq:msp_1D_delf}
    \frac{\partial f(u)}{\partial u} \biggr\rvert_{u = u_0},
\end{equation}
and $f''(u_0)$ is the second derivative of $f(u)$ evaluated at the stationary point $u_0$.

\section{\mbox{2-D} Method of Stationary Phase}
\label{subsec:msp_2D}
Similarly, for the \mbox{2-D} case, the integral,
\begin{equation}
    I(u,v) = \iint g(u,v) e^{j f(u,v)} du dv,
\end{equation}
can be approximated by
\begin{equation}
\label{eq:msp_2D}
    I(u,v) \approx \frac{g(u_0,v_0)}{\sqrt{f_{uu}f_{vv}-f^2_{uv}}} e^{j f(u_0,v_0)},
\end{equation}
where the stationary points $u_0$, $v_0$ are calculated by
\begin{gather}
\label{eq:msp_2D_delf}
    \frac{\partial f(u,v)}{\partial u} \biggr\rvert_{(u=u_0,v=v_0)} = 0, \\
    \frac{\partial f(u,v)}{\partial v} \biggr\rvert_{(u=u_0,v=v_0)} = 0,
\end{gather}
and $f_{uu}$, $f_{vv}$, $f_{uv}$ are the second partial derivatives of $f(u,v)$ evaluated at the stationary points. 

\section{Useful MSP Identities}
\label{subsec:useful_msp}
Using the aforementioned method for the \mbox{1-D} and \mbox{2-D} cases, the MSP is applied to several integrals and the corresponding approximations are provided for reference in this section.

We will demonstrate the steps for the approximation below which have been applied to the other spherical wavefronts to yield the approximations in  (\ref{eq:mspLinear})-(\ref{eq:mspCylindrical}). 

We consider the linear array case with a monostatic single antenna array being scanned along the $x$-axis at the positions labeled $x'$. Further, we consider a \mbox{1-D} target at some line $z_0$ in the $x$-$z$ plane, where the $x$ and $x'$ coordinate systems are coincident. Thus, the radar beat signal can be modeled, neglecting path loss, as
\begin{equation}
\label{eq:msp_ex1}
    s(x',k) = \int p(x) e^{j2kR} dx,
\end{equation}
where $R$ is the radial distance from each of the antenna locations $(x',0)$ to the target locations $(x,z)$ and is expressed as
\begin{equation}
    R = \sqrt{(x-x')^2 + z_0^2}.
\end{equation}

It is desired to approximate the spherical wavefront term in (\ref{eq:msp_ex1}), $e^{j2kR}$, as a more tractable expression. Thus, the MSP is exploited. For generality, the following substitutions are made $v = x'$, $r = 2k$, $w = z_0$. The \mbox{1-D} spatial Fourier transform (\ref{eq:ft1D}) is performed over the $u$ dimension of the spherical wave term and the spatial translation property (\ref{eq:ft_shiftForward}) is applied as
\begin{equation}
\label{eq:msp_ex2}
    \text{FT}_{\text{1D}}^{(u)} \left[ e^{jr\sqrt{(x-u)^2 + w^2}} \right] = e^{-jk_u x} \int e^{jr\sqrt{u^2 + w^2} - jk_u u}du.
\end{equation}

The MSP will be applied to the Fourier integral in (\ref{eq:msp_ex2}), implying for this example
\begin{gather}
    g(u) = 1, \\
    f(u) = r\sqrt{u^2 + w^2} - k_u u.
\end{gather}

Using (\ref{eq:msp_1D_delf}), the stationary point $u_0$ can be computed as 
\begin{gather}
    \frac{\partial f(u)}{\partial u} \biggr\rvert_{u = u_0} = \frac{r u_0}{\sqrt{u_0^2 + w^2}} - k_u = 0, \\
    u_0 = \frac{k_u w}{\sqrt{r^2 - k_u^2}}, \\
    f(u_0) = w\sqrt{r^2 - k_u^2}
\end{gather}

Finally, $u_0$ can be substituted into (\ref{eq:msp_1D}) ignoring the factor of $1/f''(u_0)$ as 
\begin{equation}
\label{eq:msp_ex3}
    \int e^{jr\sqrt{u^2 + w^2} - jk_u u}du \approx e^{jw\sqrt{r^2 - k_u^2}}.
\end{equation}

Substituting (\ref{eq:msp_ex3}) into (\ref{eq:msp_ex2}) yields

\begin{equation}
\label{eq:msp_ex4}
    \text{FT}_{\text{1D}}^{(u)} \left[ e^{jr\sqrt{(x-u)^2 + w^2}} \right] = e^{-jk_u x + jw\sqrt{r^2 - k_u^2}}.
\end{equation}

Taking the \mbox{1-D} inverse spatial Fourier transform of (\ref{eq:msp_ex4}) results in (\ref{eq:mspLinear}), labeled Approximation 1 below. This example illustrates the key steps of the spherical wave decomposition using the method of stationary phase. Similar analysis has been employed on the other examples below yielding the corresponding approximations using the MSP.

Approximation 1:
\begin{equation}
\label{eq:mspLinear}
    \begin{split}
        e^{jr\sqrt{(x-u)^2 + w^2}} \approx \int e^{jk_u(u-x) + j k_w w} dk_u,
    \end{split}
\end{equation}
where
\begin{equation}
    k_w^2 = r^2 - k_u^2.
\end{equation}

Approximation 2:
\begin{equation}
\label{eq:mspRectilinear}
    \begin{split}
        &\frac{e^{jr\sqrt{(x-u)^2 + (y-v)^2 + w^2}}}{\sqrt{(x-u)^2 + (y-v)^2 + w^2}} \\
        & \approx \iint \frac{1}{k_w} e^{jk_u(u-x) + jk_v(v-y) + k_w w} dk_u dk_v,
    \end{split}
\end{equation}
where
\begin{equation}
    k_w^2 = r^2 - k_u^2 - k_v^2.
\end{equation}

Approximation 3:
\begin{equation}
\label{eq:mspCircular}
    \begin{split}
        e^{jr\sqrt{(x-u)^2 + (z-w)^2}} \approx \iint e^{jk_u(u-x) + j k_w (w-z)} dk_u dk_w.
    \end{split}
\end{equation}

Approximation 4:
\begin{equation}
\label{eq:mspCylindrical}
    \begin{split}
        & e^{jr\sqrt{(x-u)^2 + (y-v)^2 + (z-w)^2}} \\
        & \approx \iiint e^{jk_u(u-x) + jk_v(v-y) + jk_w(w-z)} dk_u dk_v dk_w.
    \end{split}
\end{equation}
