# Supplementary material for: Novel Hybrid-Learning Algorithms for Improved Millimeter-Wave Imaging Systems
Source: arXiv:2306.15341 source file (2023-06-27)
Supplement: Supplementary file 3 [file appendixZ.tex]

\chapter{Efficient Near-Field SAR Image Reconstruction Algorithms for Various Geometries}
\label{app:reconstruction_algos}

\section{\mbox{1-D} Linear Synthetic Array \mbox{1-D} Imaging - Fourier-based}
\label{app:linear_fft}
In this section, we derive the image reconstruction algorithm for recovering a \mbox{1-D} reflectivity function from a \mbox{1-D} linear SAR scenario in the near-field. Given a \mbox{1-D} linear SISO synthetic array whose elements are located at the points $(y',Z_0)$ in the $y$-$z$ plane and a \mbox{1-D} target with reflectivity function $p(y)$ located at the points $(y,z_0)$, the isotropic beat signal can be written as
\begin{equation}
\label{eq:linear_fft1}
    s(y',k) = \int \frac{p(y)}{R^2} e^{j2kR} dy,
\end{equation}
where
\begin{equation}
    R = \sqrt{(y-y')^2 + (z_0 - Z_0)^2}.
\end{equation}
Ignoring amplitude terms, applying the MSP derived in (\ref{eq:mspLinear}), the spherical phase term in (\ref{eq:linear_fft1}) can be substituted yielding
\begin{equation}
\label{eq:linear_fft2}
    s(y',k) = \iint p(y) e^{j(k_y'(y'-y) + k_z(z_0-Z_0))}dy dk_y', 
\end{equation}
where
\begin{equation}
    k_z = \sqrt{4k^2 - k_y^2}.
\end{equation}
Rearranging the phase terms in (\ref{eq:linear_fft2}), a forward spatial Fourier transform on $y$ and inverse spatial Fourier transform on $y'$ become evident as
\begin{gather}
    s(y',k) = \int  \left[ \int p(y)e^{-jk_y'y}dy \right] e^{j(k_y'y'+ k_z(z_0-Z_0))} dk_y'.
\end{gather}
The term inside the brackets can be rewritten as the spatial-spectral representation of the target reflectivity function, $P(k_y)$. Then, performing a forward Fourier transform along $y'$ on both sides simplifies the expression as the following. Note that the distinction between the primed and unprimed domains can be dropped in the spatial Fourier domain as they coincide.
\begin{gather}
    s(y',k) = \int \left[ P(k_y)  e^{jk_z(z_0-Z_0)} \right] e^{jk_y'y'} dk_y', \\
    S(k_y,k) = P(k_y)e^{jk_z(z_0-Z_0)}, \\
    P(k_y) = S(k_y,k)e^{-jk_z(z_0-Z_0)}.
    \label{eq:linear_fft3}
\end{gather}

For wideband waveforms, (\ref{eq:linear_fft3}) is evaluated at multiple wavenumbers thus coherent summation is performed over $k$. 
Hence, the complete expression for the Fourier-based \mbox{1-D} image reconstruction algorithm for a \mbox{1-D} linear SISO synthetic array is
\begin{equation}
\label{eq:linear_fft_final}
    p(y) = \int \text{IFT}_{\text{1D}}^{(k_y)} \left[ \text{FT}_{\text{1D}}^{(y')} [s(y',k)] e^{-jk_z(z_0-Z_0)} \right]dk.
\end{equation}

\section{\mbox{1-D} Linear Synthetic Array \mbox{2-D} Imaging - Range Migration Algorithm}
\label{app:linear_rma}
In this section we derive the image reconstruction algorithm for recovering a \mbox{2-D} reflectivity function from a \mbox{1-D} linear SAR scenario in the near-field. Given a \mbox{1-D} linear SISO synthetic array whose elements are located at the points $(y',Z_0)$ in the $y$-$z$ plane and a \mbox{2-D} target with reflectivity function $p(y,z)$ located at the points $(y,z)$, the isotropic beat signal can be written as
\begin{equation}
\label{eq:linear_rma1}
    s(y',k) = \iint \frac{p(y,z)}{R^2} e^{j2kR} dy dz,
\end{equation}
where
\begin{equation}
    R = \sqrt{(y-y')^2 + (z - Z_0)^2}.
\end{equation}
Ignoring amplitude terms, applying the MSP derived in (\ref{eq:mspLinear}), the spherical phase term in (\ref{eq:linear_rma1}) can be substituted yielding
\begin{equation}
\label{eq:linear_rma2}
    s(y',k) = \iiint p(y,z) e^{j(k_y'(y'-y) + k_z(z-Z_0))}dy dz dk_y', 
\end{equation}
where
\begin{equation}
    k_z = \sqrt{4k^2 - k_y^2}.
\end{equation}
Leveraging conjugate symmetry of the spherical wavefront, (\ref{eq:linear_rma2}) can be rewritten in the following form to exploit the spatial Fourier transform on $z$
\begin{equation}
\label{eq:linear_rma3}
    s^*(y',k) = \iiint p(y,z) e^{j(k_y'(y'-y) - k_z(z-Z_0))}dy dz dk_y', 
\end{equation}
where $(\bullet)^*$ is the complex conjugate operation.

Rearranging the phase terms in (\ref{eq:linear_rma3}), a forward spatial Fourier transform on $y$-$z$ and inverse spatial Fourier transform on $y'$ become evident as
\begin{equation}
    \begin{split}
        s^*(y',k) &= \int  \left[ \iint p(y,z)e^{-j(k_y'y+k_z z)}dydz \right] \\
        & \times e^{j(k_y'y'+ k_z Z_0)} dk_y'.
    \end{split}
\end{equation}
The term inside the brackets can be rewritten as the spatial-spectral representation of the target reflectivity function, $P(k_y,k_z)$. Then, performing a forward Fourier transform along $y'$ on both sides simplifies the expression as the following. Note that the distinction between the primed and unprimed domains can be dropped in the spatial Fourier domain as they coincide.
\begin{gather}
    s^*(y',k) = \int \left[ P(k_y,k_z)  e^{jk_z Z_0} \right] e^{jk_y'y'} dk_y', \\
    \Tilde{S}(k_y,k) = \text{FT}_{\text{1D}}^{(y')} [s^*(y',k)], \\
    \Tilde{S}(k_y,k) = P(k_y,k_z)e^{jk_z Z_0}, \\
    P(k_y,k_z) = \Tilde{S}(k_y,k)e^{-jk_z Z_0}.
    \label{eq:linear_rma4}
\end{gather}

The direct relationship between $P(k_y,k_z)$ and $\Tilde{S}(k_y,k)$ is now obvious in (\ref{eq:linear_rma4}); however, $P(k_y,k_z)$ is sampled on a uniform $k_y$-$k_z$ grid and $\Tilde{S}(k_y,k)$ is sampled on a uniform $k_y$-$k$ grid. Before the reflectivity function can be recovered using in inverse Fourier transform, $\Tilde{S}(k_y,k)e^{-jk_z Z_0}$ must be interpolated to a uniform $k_y$-$k_z$ grid using Stolt interpolation, represented by the $\mathcal{S}[\bullet]$ operator, to account for the curvature of the wavefront \cite{lopez20003}.
\begin{equation}
    S(k_y,k_z) = \mathcal{S} \left[ \Tilde{S}(k_y,k)e^{-jk_z Z_0} \right].
\end{equation}

Finally, the complete expression for the Fourier-based \mbox{2-D} image reconstruction algorithm for a \mbox{1-D} linear SISO synthetic array can be written as
\begin{equation}
\label{eq:linear_rma_final}
    p(y,z) = \text{IFT}_{\text{2D}}^{(k_y,k_z)}  \left[ \mathcal{S} \left[ \text{FT}_{\text{1D}}^{(y')} [s^*(y',k)] e^{-jk_z Z_0} \right] \right].
\end{equation}

\section{\mbox{2-D} Rectilinear Array \mbox{2-D} Imaging - Fourier-based}
\label{app:rectilinear_fft}
In this section, we derive the image reconstruction algorithm for recovering a \mbox{2-D} reflectivity function from a \mbox{2-D} rectilinear SAR scenario in the near-field \cite{paul2021systematic,yanik2019sparse,yanik2019near}. Given a \mbox{2-D} rectilinear SISO synthetic array whose elements are located at the points $(x',y',Z_0)$ in $x$-$y$-$z$ space and a \mbox{2-D} target with reflectivity function $p(x,y)$ located at the points $(x,y,z_0)$, the isotropic beat signal can be written as
\begin{equation}
\label{eq:rectilinear_fft1}
    s(x',y',k) = \iint \frac{p(x,y)}{R^2} e^{j2kR} dx dy,
\end{equation}
where
\begin{equation}
    R = \sqrt{(x-x')^2 + (y-y')^2 + (z_0 - Z_0)^2}.
\end{equation}
Assuming the points of the target scene are closely located, the $R^{-2}$ factor in (\ref{eq:rectilinear_fft1}) can be approximated as $R^{-1}$ \cite{yanik2019sparse}. Applying the MSP derived in (\ref{eq:mspRectilinear}), the spherical phase term in (\ref{eq:rectilinear_fft1}) can be substituted yielding
\begin{equation}
\label{eq:rectilinear_fft2}
    \begin{split}
        s(x',y',k) &= \iiiint \frac{p(x,y)}{k_z} e^{j(k_x'(x'-x) + k_y'(y'-y))} \\
        & \times e^{jk_z(z_0-Z_0)}dx dy dk_x' dk_y', 
    \end{split}
\end{equation}
where
\begin{equation}
    k_z = \sqrt{4k^2 - k_x^2 - k_y^2}.
\end{equation}
Rearranging the phase terms in (\ref{eq:rectilinear_fft2}), a forward spatial Fourier transform on $x$-$y$ and inverse spatial Fourier transform on $x'$-$y'$ become evident as
\begin{equation}
    \begin{split}
        s(x'y',k) &= \iint  \left[ \iint \frac{p(x,y)}{k_z} e^{-j(k_x'x + k_y'y)}dx dy \right] \\
        & \times e^{j(k_x'x' + k_y'y')+ jk_z(z_0-Z_0)} dk_x' dk_y'.
    \end{split}
\end{equation}
The term inside the brackets can be rewritten as the spatial-spectral representation of the target reflectivity function. Then, performing a forward Fourier transform along $x'$-$y'$ on both sides simplifies the expression as the following. Note that the distinction between the primed and unprimed domains can be dropped in the spatial Fourier domain as they coincide.
\begin{equation}
    \begin{split}
        s(x',y',k) &= \int \left[ \frac{P(k_x,k_y)}{k_z}  e^{jk_z(z_0-Z_0)} \right] \\
        & \times e^{j(k_x'x' + k_y'y')}dk_x' dk_y', \\
    \end{split}
\end{equation}
\begin{gather}
    S(k_x,k_y,k) = \frac{P(k_x,k_y)}{k_z}e^{jk_z(z_0-Z_0)}, \\
    P(k_x,k_y) = S(k_y,k)k_z e^{-jk_z(z_0-Z_0)}.
    \label{eq:rectilinear_fft3}
\end{gather}

For wideband waveforms, (\ref{eq:rectilinear_fft3}) is evaluated at multiple wavenumbers thus coherent summation is performed over $k$. 
Hence, the complete expression for the Fourier-based \mbox{2-D} image reconstruction algorithm for a \mbox{2-D} rectilinear SISO synthetic array is
\begin{equation}
\label{eq:rectilinear_fft_final}
    \begin{split}
        p(x,y) &= \int \text{IFT}_{\text{2D}}^{(k_x,k_y)} \biggr[ \text{FT}_{\text{2D}}^{(x',y')} [s(x',y',k)] \\
        & \times k_z e^{-jk_z(z_0-Z_0)} \biggr] dk.
    \end{split}
\end{equation}

\section{\mbox{2-D} Rectilinear Array \mbox{3-D} Imaging -  Range Migration Algorithm}
\label{app:rectilinear_rma}
In this section we derive the image reconstruction algorithm for recovering a \mbox{3-D} reflectivity function from a \mbox{2-D} rectilinear SAR scenario in the near-field. Given a \mbox{2-D} rectilinear SISO synthetic array whose elements are located at the points $(x',y',Z_0)$ in $x$-$y$-$z$ space and a \mbox{3-D} target with reflectivity function $p(x,y,z)$ located at the points $(x,y,z)$, the isotropic beat signal can be written as
\begin{equation}
\label{eq:rectilinear_rma1}
    s(x',y',k) = \iiint \frac{p(x,y,z)}{R^2} e^{j2kR} dx dy dz,
\end{equation}
where
\begin{equation}
    R = \sqrt{(x-x')^2 + (y-y')^2 + (z - Z_0)^2}.
\end{equation}
Assuming the points of the target scene are closely located, the $R^{-2}$ factor in (\ref{eq:rectilinear_rma1}) can be approximated as $R^{-1}$ \cite{yanik2019sparse}. 
Applying the MSP derived in (\ref{eq:mspRectilinear}), the spherical phase term in (\ref{eq:rectilinear_rma1}) can be substituted yielding
\begin{equation}
\label{eq:rectilinear_rma2}
    \begin{split}
        s(x',y',k) &= \iint \biggr[ \iiint p(x,y,z) e^{j(k_x'(x'-x) + k_y'(y'-y))} \\
        & \times e^{jk_z(z-Z_0)}dx dy dz \biggr] dk_x' dk_y', 
    \end{split}
\end{equation}
where
\begin{equation}
    k_z = \sqrt{4k^2 - k_x^2 - k_y^2}.
\end{equation}
Leveraging conjugate symmetry of the spherical wavefront, (\ref{eq:rectilinear_rma2}) can be rewritten in the following form to exploit the spatial Fourier transform on $z$
\begin{equation}
\label{eq:rectilinear_rma3}
    \begin{split}
        s^*(x',y',k) &= \iint \biggr[ \iiint p(x,y,z) e^{j(k_x'(x'-x) + k_y'(y'-y))} \\
        & \times e^{-jk_z(z-Z_0)}dx dy dz \biggr] dk_x' dk_y', 
    \end{split}
\end{equation}
where $(\bullet)^*$ is the complex conjugate operation.

Rearranging the phase terms in (\ref{eq:rectilinear_rma3}), a forward spatial Fourier transform on $x$,$y$,$z$ and inverse spatial Fourier transform on $x'$,$y'$ become evident as
\begin{equation}
    \begin{split}
        s^*(x',y',k) &= \iint  \biggr[ \iiint p(x,y,z)e^{-(jk_x' x + jk_y' y + jk_z z)} \\
        & \times dxdydz \biggr] e^{j(k_x'x'+k_y'y')+ jk_z Z_0} dk_x' dk_y'.
    \end{split}
\end{equation}
The term inside the brackets can be rewritten as the spatial-spectral representation of the target reflectivity function. Then, performing a forward Fourier transform along $x'$, $y'$ on both sides simplifies the expression as the following. Note that the distinction between the primed and unprimed domains can be dropped in the spatial Fourier domain as they coincide.
\begin{equation}
    \begin{split}
        s^*(x',y',k) &= \int \left[ P(k_x,k_y,k_z)  e^{jk_z Z_0} \right] \\
        & \times e^{j(k_x'x'+k_y'y')} dk_x' dk_y', \\
    \end{split}
\end{equation}

\begin{gather}
    \Tilde{S}(k_x,k_y,k) = \text{FT}_{\text{2D}}^{(x',y')} [s^*(x',y',k)], \\
    \Tilde{S}(k_x,k_y,k) = P(k_x,k_y,k_z)e^{jk_z Z_0}, \\
    P(k_x,k_y,k_z) = \Tilde{S}(k_x,k_y,k)e^{-jk_z Z_0}.
    \label{eq:rectilinear_rma4}
\end{gather}

The direct relationship between $P(k_x,k_y,k_z)$ and $\Tilde{S}(k_x,k_y,k)$ is now obvious in (\ref{eq:rectilinear_rma4}); however, $P(k_x,k_y,k_z)$ is sampled on a uniform $k_x$-$k_y$-$k_z$ grid and $\Tilde{S}(k_x,k_y,k)$ is sampled on a uniform $k_x$-$k_y$-$k$ grid. 
Before the reflectivity function can be recovered using an inverse Fourier transform, $\Tilde{S}(k_x,k_y,k)e^{-jk_z Z_0}$ must be interpolated to a uniform $k_x,k_y$-$k_z$ grid using the Stolt interpolation, represented by the $\mathcal{S}[\bullet]$ operator, to account for the curvature of the wavefront \cite{lopez20003}.
\begin{equation}
    S(k_x,k_y,k_z) = \mathcal{S} \left[ \Tilde{S}(k_x,k_y,k)e^{-jk_z Z_0} \right].
\end{equation}

Finally, the complete expression for the Fourier-based \mbox{3-D} image reconstruction algorithm for a \mbox{2-D} rectilinear SISO synthetic array can be written as
\begin{equation}
\label{eq:rectilinear_rma_final}
    \begin{split}
        p(x,y,z) &= \text{IFT}_{\text{3D}}^{(k_x,k_y,k_z)}  \biggr[ \mathcal{S} \biggr[ \text{FT}_{\text{2D}}^{(x',y')} [s^*(x',y',k)] \\
        & \times e^{-jk_z Z_0} \biggr] \biggr].
    \end{split}
\end{equation}

\section{\mbox{1-D} Circular Synthetic Array \mbox{2-D} Imaging - Polar Formatting Algorithm}
\label{app:circular_pfa}
In this section, we derive the image reconstruction algorithm for recovering a \mbox{2-D} reflectivity function from a \mbox{1-D} circular SAR scenario in the near-field. Given a \mbox{1-D} circular SISO synthetic array whose elements are located at the points $(R_0\cos\theta,R_0\sin\theta)$ in the $x$-$z$ plane at $y = 0$, where $R_0$ and $\theta$ are the constant radial distance from the antenna elements to the origin and the angular dimension, respectively, and a \mbox{2-D} target with reflectivity function $p(x,z)$ located at the points $(x,z)$, the isotropic beat signal can be written as
\begin{equation}
\label{eq:circular_pfa1}
    s(\theta,k) = \iint \frac{p(x,z)}{R^2} e^{j2kR} dx dz,
\end{equation}
where
\begin{equation}
    R = \sqrt{(x-R_0\cos\theta)^2 + (z-R_0\sin\theta)^2}.
\end{equation}

The MSP derived in (\ref{eq:mspCircular}) can be applied to the spherical phase term in (\ref{eq:circular_pfa1}) after the following substitutions
\begin{gather}
\label{eq:circular_pfa_sub1}
    x' = R_0\cos\theta, \\
    z' = R_0\cos\theta, \\
    k_x' = k_r \cos\alpha, \\
    k_z' = k_r \cos\alpha, \\
    k_r^2 = k_x'^2 + k_z'^2,
    \label{eq:circular_pfa_subEnd}
\end{gather}
yielding
\begin{gather}
\label{eq:circular_pfa2}
    e^{j2kR} \approx \iint e^{j(k_x'(x'-x) + k_z'(z'-z))} dk_x' dk_z'.
\end{gather}

Neglecting path loss, (\ref{eq:circular_pfa1}) and (\ref{eq:circular_pfa2}) can be combined as
\begin{equation}
\label{eq:circular_pfa3}
    s(\theta,k) = \iiiint p(x,z) e^{j(k_x'(x'-x) + k_z'(z'-z))} dx dz dk_x' dk_z'.
\end{equation}

Rearranging the phase terms in (\ref{eq:circular_pfa3}), a forward spatial Fourier transform on $x$-$z$ and inverse spatial Fourier transform on $x'$-$z'$ become evident as
\begin{equation}
\label{eq:circular_pfa4}
    \begin{split}
        s(\theta,k) &= \iint  \left[ \iint p(x,z) e^{-j(k_x'x + k_z'z)}dx dz \right] \\
        & \times e^{j(k_x'x' + k_z'z')} dk_x' dk_z'.
    \end{split}
\end{equation}

The term inside the brackets can be rewritten as the spatial spectral representation of the target reflectivity function, $P(k_x,k_z)$. Then using the relations (\ref{eq:circular_pfa_sub1})-(\ref{eq:circular_pfa_subEnd}), the expression in (\ref{eq:circular_pfa4}) can be rewritten as
\begin{equation}
    \begin{split}
        s(\theta,k) &= \iint  P(k_x,k_z) e^{j(k_r\cos\theta R_0\cos\alpha + k_r\sin\theta R_0\sin\alpha)} \\
        & \times k_r dk_r d\alpha.
    \end{split}
\end{equation}

Rewriting the spectral $P(k_x,k_z)$ as its equivalent spectral polar form $P(\alpha,k_r)$ and simplifying the phase term
\begin{equation}
\label{eq:circular_pfa5}
    s(\theta,k) = \int \biggr[ \int P(\alpha,k_r) e^{jk_r R_0 cos(\theta - \alpha)} d\alpha \biggr] k_r dk_r.
\end{equation}

The term inside the brackets in (\ref{eq:circular_pfa5}) is a convolution operation in the $\theta$ domain, where the $\theta$ and $\alpha$ domains are coincident and can be exploited using Fourier relations by taking a Fourier transform across $\theta$ on both sides of the equation as 
\begin{equation}
\label{eq:circular_pfa6}
    S(k_\theta,k) = \int P(k_\theta,k_r) \times \text{FT}_{\text{1D}}^{(\theta)} \left[ e^{jk_r R_0 \cos\theta} \right] k_r dk_r.
\end{equation}

Considering only the values lying on the Ewald sphere, $k_r^2 = 4k^2$ imposes a $\delta$-function behavior of the integrand in (\ref{eq:circular_pfa6}) with respect to $k_r$ \cite{amineh2019real}.
As such, (\ref{eq:circular_pfa6}) can be simplified as such, substituting $k_r = 2k$,
\begin{equation}
\label{eq:circular_pfa7}
    P(k_\theta,k_r) = S(k_\theta,k)G^*(k_\theta,k),
\end{equation}
where
\begin{equation}
\label{eq:circular_pfa_G}
    G(k_\theta,k) = \text{FT}_{\text{1D}}^{(\theta)} \left[ e^{j2 k R_0 \cos\theta} \right].
\end{equation}

The spatial spectral reflectivity function in polar coordinates can be recovered from (\ref{eq:circular_pfa7}) as 
\begin{equation}
    P(\theta,k_r) = \text{IFT}_{\text{1D}}^{(k_\theta)} \left[ S(k_\theta,k)G^*(k_\theta,k) \right].
\end{equation}

Finally, the reflectivity function $p(x,z)$ can be recovered using a nonuniform FFT (NUFFT) \cite{gao2016efficient} or via interpolation to the rectangular spatial Fourier domain $k_x$-$k_z$ followed by a uniform IFFT. This interpolation operation, known as the polar formatting algorithm (PFA), is denoted by $\mathcal{P}[\bullet]$. Thus, the final step in the image recovery process is (prime notation will be ignored for the remainder of this derivation as the primed and unprimed coordinate systems are coincident)
\begin{equation}
    p(x,z) = \text{IFT}_{\text{2D}}^{(k_x,k_z)} \left[ \mathcal{P}[P(\theta,k_r)] \right].
\end{equation}

Finally, the complete expression for the Fourier-based \mbox{2-D} image reconstruction algorithm for a \mbox{1-D} circular SISO synthetic array can be written as
\begin{equation}
\label{eq:circular_pfa_final}
    \begin{split}
        p(x,z) &= \text{IFT}_{\text{2D}}^{(k_x,k_z)} \biggr[ \mathcal{P}\biggr[ \text{IFT}_{\text{1D}}^{(k_\theta)} \biggr[ S(k_\theta,k) \\
        & \times \text{FT}_{\text{1D}}^{(\theta)} \biggr[ e^{j2 k R_0 \cos\theta} \biggr]^* \biggr] \biggr] \biggr].
    \end{split}
\end{equation}

\section{\mbox{2-D} Cylindrical Synthetic Array \mbox{3-D} Imaging - Polar Formatting Algorithm}
\label{app:cylindrical_pfa}
In this section, we derive the image reconstruction algorithm for recovering a \mbox{3-D} reflectivity function from a \mbox{2-D} cylindrical SAR (also known as ECSAR) scenario in the near-field. Given a \mbox{2-D} cylindrical SISO synthetic array whose elements are located at the points $(R_0\cos\theta,y',R_0\sin\theta)$ in $x$-$y$-$z$ space, where $R_0$ and $\theta$ are the constant radial distance from the antenna elements to the origin and the angular dimension, respectively, and a \mbox{3-D} target with reflectivity function $p(x,y,z)$ located at the points $(x,y,z)$, the isotropic beat signal can be written as
\begin{equation}
\label{eq:cylindrical_pfa1}
    s(\theta,y',k) = \iiint \frac{p(x,y,z)}{R^2} e^{j2kR} dx dy dz,
\end{equation}
where
\begin{equation}
    R = \sqrt{(x-R_0\cos\theta)^2 + (y-y')^2 + (z-R_0\sin\theta)^2}.
\end{equation}

The MSP derived in (\ref{eq:mspCylindrical}) can be applied to the spherical phase term in (\ref{eq:cylindrical_pfa1}) after the following substitutions
\begin{gather}
\label{eq:cylindrical_pfa_sub1}
    x' = R_0\cos\theta, \\
    z' = R_0\cos\theta, \\
    k_x' = k_r \cos\alpha, \\
    k_z' = k_r \cos\alpha, \\
    k_r^2 = k_x'^2 + k_z'^2 = 4k^2 - k_y'^2,
    \label{eq:cylindrical_pfa_subEnd}
\end{gather}
yielding
\begin{gather}
\label{eq:cylindrical_pfa2}
    e^{j2kR} \approx \iint e^{j(k_x'(x'-x) + k_y'(y'-y) + k_z'(z'-z))} dk_x' dk_y' dk_z'.
\end{gather}

Neglecting path loss, (\ref{eq:cylindrical_pfa1}) and (\ref{eq:cylindrical_pfa2}) can be combined as
\begin{equation}
\label{eq:cylindrical_pfa3}
    \begin{split}
        s(\theta,y',k) &= \iiint \biggr[ \iiint p(x,y,z)  \\
         & \times e^{j(k_x'(x'-x)+ k_y'(y'-y) + k_z'(z'-z))} \\
         & \times dx dy dz \biggr] dk_x' dk_y' dk_z'.
    \end{split}
\end{equation}

Rearranging the phase terms in (\ref{eq:cylindrical_pfa3}), a forward spatial Fourier transform on $x$-$y$-$z$ and inverse spatial Fourier transform on $x'$-$y'$-$z'$ become evident as
\begin{equation}
\label{eq:cylindrical_pfa4}
    \begin{split}
        s(\theta,y',k) &= \iiint  \left[ \iiint p(x,y,z) e^{-j(k_x'x + k_y'y + k_z'z)}dx dy dz \right] \\
        & \times e^{j(k_x'x' + k_y'y' + k_z'z')} dk_x' dk_y' dk_z'.
    \end{split}
\end{equation}

The term inside the brackets can be rewritten as the spatial spectral representation of the target reflectivity function, $P(k_x,k_y,k_z)$. Then using the relations (\ref{eq:cylindrical_pfa_sub1})-(\ref{eq:cylindrical_pfa_subEnd}), the expression in (\ref{eq:cylindrical_pfa4}) can be rewritten as
\begin{equation}
    \begin{split}
        s(\theta,y',k) &= \iiint  P(k_x,k_y,k_z) e^{j(k_r\cos\theta R_0\cos\alpha} \\
        & \times e^{j(k_r\sin\theta R_0\sin\alpha) + k_y'y')} k_r dk_y' dk_r d\alpha.
    \end{split}
\end{equation}

Taking a Fourier transform on both side with respect to $y'$, rewriting the spectral $P(k_x,k_y,k_z)$ as its equivalent spectral polar form $P(\alpha,k_y,k_r)$, and simplifying the phase term yields (prime notation will be dropped for the remainder of this derivation as the primed and unprimed coordinate systems are coincident)
\begin{equation}
\label{eq:cylindrical_pfa5}
    s(\theta,k_y,k) = \int \biggr[ \int P(\alpha,k_y,k_r) e^{jk_r R_0 cos(\theta - \alpha)} d\alpha \biggr] k_r dk_r.
\end{equation}

The term inside the brackets in (\ref{eq:cylindrical_pfa5}) is a convolution operation in the $\theta$ domain, where the $\theta$ and $\alpha$ domains are coincident and can be exploited using Fourier relations by taking a Fourier transform across $\theta$ on both sides of the equation as 
\begin{equation}
\label{eq:cylindrical_pfa6}
    S(k_\theta,k_y,k) = \int P(k_\theta,k_y,k_r) \text{FT}_{\text{1D}}^{(\theta)} \left[ e^{jk_r R_0 \cos\theta} \right] k_r dk_r.
\end{equation}

Considering only the values lying on the Ewald sphere, $k_r^2 = 4k^2 - k_y^2$ imposes a $\delta$-function behavior of the integrand in (\ref{eq:cylindrical_pfa6}) with respect to $k_r$ \cite{amineh2019real}.
As such, (\ref{eq:cylindrical_pfa6}) can be simplified as such, substituting $k_r = \sqrt{4k^2 - k_y^2}$,
\begin{equation}
\label{eq:cylindrical_pfa7}
    P(k_\theta,k_y,k_r) = S(k_\theta,k_y,k)G^*(k_\theta,k_y,k),
\end{equation}
where
\begin{equation}
\label{eq:cylindrical_pfa_G}
    G(k_\theta,k_y,k) = \text{FT}_{\text{1D}}^{(\theta)} \left[ e^{j \sqrt{4k^2 - k_y^2} R_0 \cos\theta} \right].
\end{equation}

The spatial spectral reflectivity function in polar coordinates can be recovered from (\ref{eq:cylindrical_pfa7}) as 
\begin{equation}
    P(\theta,k_y,k_r) = \text{IFT}_{\text{1D}}^{(k_\theta)} \left[ S(k_\theta,k_y,k)G^*(k_\theta,k_y,k) \right].
\end{equation}

Finally, the reflectivity function $p(x,y,z)$ can be recovered using a nonuniform FFT (NUFFT) \cite{gao2016efficient} or via interpolation to the rectangular spatial Fourier domain $k_x$-$k_y$-$k_z$ followed by a uniform IFFT. This interpolation operation, known as the polar formatting algorithm (PFA), is denoted by $\mathcal{P}[\bullet]$. Thus, the final step in the image recovery process is
\begin{equation}
    p(x,y,z) = \text{IFT}_{\text{3D}}^{(k_x,k_y,k_z)} \left[ \mathcal{P}[P(\theta,k_y,k_r)] \right].
\end{equation}

Finally, the complete expression for the Fourier-based \mbox{3-D} image reconstruction algorithm for a \mbox{2-D} cylindrical SISO synthetic array can be written as
\begin{equation}
\label{eq:cylindrical_pfa_final}
    \begin{split}
        p(x,y,z) &= \text{IFT}_{\text{3D}}^{(k_x,k_y,k_z)} \biggr[ \mathcal{P}\biggr[ \text{IFT}_{\text{1D}}^{(k_\theta)} \biggr[ S(k_\theta,k_y,k) \\
        & \times \text{FT}_{\text{1D}}^{(\theta)} \biggr[ e^{j \sqrt{4k^2 - k_y^2} R_0 \cos\theta} \biggr]^* \biggr] \biggr] \biggr].
    \end{split}
\end{equation}
